# Supplementary material for: D3VO: Deep Depth, Deep Pose and Deep Uncertainty for Monocular Visual Odometry
Source: arXiv:2003.01060 source file (2020-03-28)
Supplement: Supplementary file 1 [file main_supp.tex]

\input{settings.tex}

\begin{document}
\setlength{\abovedisplayskip}{3pt}
\setlength{\belowdisplayskip}{3pt}
	
\title{\ $\text{D}^\text{3}$VO: Deep Depth, Deep Pose and Deep Uncertainty\\
	for Monocular Visual Odometry\\
	\underline{Supplementary Material}}
\author{First Author\\
Institution1\\
Institution1 address\\
{\tt\small firstauthor@i1.org}
\and
Second Author\\
Institution2\\
First line of institution2 address\\
{\tt\small secondauthor@i2.org}
}

\maketitle

\input{sections/supp/2_train.tex}

\input{sections/supp/3_net_arch.tex}

\input{sections/supp/4_add_ab.tex}

\input{sections/supp/5_cs_exp.tex}

\clearpage
{\small
\bibliographystyle{ieee_fullname}
\bibliography{egbib_supp}
}

\end{document}
